# Supplementary material for: FIRM: An Intelligent Fine-Grained Resource Management Framework for SLO-Oriented Microservices
Source: arXiv:2008.08509 source file (2020-10-19)
Supplement: Supplementary file 1 [file 01000-appendix.tex]

\appendix
\section{Artifact Appendix}
\subsection{Abstract}
\xxx is publicly available at \url{https://gitlab.engr.illinois.edu/DEPEND/firm.git}.
We provide implementations for FIRM's SVM-based critical component extraction, RL-based SLO violation mitigation, and the performance anomaly injection.
In addition, we provide a tracing data set of the four microservice benchmarks deployed on our dedicated Kubernetes cluster of 15 physical nodes.
The data set was generated by running open-loop workload generation and performance anomaly injection.

\subsection{Artifact Check-list}
\begin{small}
\begin{itemize}
  \item {\bf Algorithm: }\xxx's critical component extraction includes an algorithm to find the weighted longest path (i.e., critical path analysis) from the execution history graph of microservices.
  \item {\bf Model: }\xxx's two-level machine learning architecture includes an SVM-based critical component extraction model and an RL-based SLO violation mitigation model. The latter one is designed based on deep deterministic policy gradient (DDPG).
  \item {\bf Data set: }The artifact includes a tracing data set collected by running four microservice benchmarks~\cite{gan2019open,traintickets} in a 15-node Kubernetes cluster. The microservice benchmarks are driven by workload generation and performance anomaly injection.
  \item {\bf Hardware: }Experiments can run on a cluster of physical nodes with Intel Cache Allocation Technology (CAT)~\cite{intelcat} and Intel Memory Bandwidth Allocation (MBA)~\cite{intelmba} enabled.
  \item {\bf Required disk space: }Neo4j~\cite{neo4j} requires 10 GB minimum block storage, and the storage size depends on the size of the database.
  \item {\bf Set-up instructions: }Set-up instructions are available at the \texttt{README.md} file in the repository.
  \item {\bf Public link: }\url{https://gitlab.engr.illinois.edu/DEPEND/firm.git}
  \item {\bf Code licenses: }Apache License Version 2.0
  \item {\bf Data licenses: }CC0 License
\end{itemize}
\end{small}

\subsection{Description}
\subsubsection{How to Access}
The artifact is publicly available at \url{https://gitlab.engr.illinois.edu/DEPEND/firm.git}.

\subsubsection{Hardware Dependencies}
Experiments can be run on a cluster of physical nodes with processors that have Intel CAT and MBA technologies enabled.
They are required for last-level cache partitioning and memory bandwidth partitioning respectively.

\subsubsection{Software Dependencies}
Software dependencies are specified at the \texttt{README.md} file, which includes Kubernetes, Docker-Compose, and Docker.

\subsubsection{Data Sets}
The tracing data sets of four microservice benchmarks deployed on our dedicated Kubernetes cluster consisting of 15 heterogeneous nodes are also available.
The data sets are not sampled and are from selected types of requests in each benchmark, i.e., compose-posts in the social network application, compose-reviews in the media service application, book-rooms in the hotel reservation application, and reserve-tickets in the train ticket booking application.
A detailed description is available at \texttt{data/README.md}.

%\subsubsection{Models}
%Models of FIRM's RL-based SLO violation mitigation are available at \texttt{ddpg/} while alternative RL models are also available at \texttt{rl-alts/}.

\subsection{Installation}
Installation instructions are specified at the \texttt{README.md} file in the repository.

\subsection{Experiment Workflow}
Experiments on physical clusters start from deploying the Kubernetes with FIRM.
Microservice applications instrumented with the OpenTracing~\cite{opentracing} standard are then deployed in the Kubernetes cluster.
One can also use the instrumented microservice benchmarks in the repository for experiments.
To drive the experiments, workload generators and performance anomaly injectors should be configured and installed accordingly.
Then the training of FIRM's ML models is divided into two phases.
In the first phase, the workflow stops at the SLO violation localization.
The SVM model is trained with the feature data retrieved from the tracing coordinator and the label data from the performance anomaly injection campaign.
In the second phase, the workflow continues and FIRM's RL agent is trained by interacting with the environment.

\subsection{Experiment Customization}
FIRM's multilevel ML modeling provides the flexibility of customizing the algorithms for both SLO violation localization and mitigation.
The SVM model can be replaced by other supervised learning models or other heuristics-based methods.
The DDPG algorithm used by the RL agent can also be replaced by other RL algorithms.
The repository consists of the implementations of other alternative RL models such as proximal policy optimization (PPO) and policy gradient.

In addition, different types of resources in control are also configurable in the RL agent and the performance anomaly injector.
That pluggability allows one to add or remove resources, and to change the actions associated with each type of resource.

\subsection{AE Methodology}

Submission, reviewing and badging methodology:

\begin{itemize}
  \item \url{https://www.usenix.org/conference/osdi20/call-for-artifacts}
\end{itemize}
